# Supplementary material for: On the Implicit Bias of Gradient Descent for Temporal Extrapolation
Source: arXiv:2202.04302 source file (2022-03-24)
Supplement: Supplementary file 1 [file supplement.tex]

\documentclass[twoside]{article}

% \usepackage{aistats2022}
\usepackage{amsfonts, amsthm}
\usepackage{graphicx}
\usepackage{xcolor}         % colors
\newcommand{\amirg}[1]{\textcolor{red}{Amir: #1}}
\newcommand{\comment}[1]{}
\newcommand{\nadav}[1]{\textcolor{blue}{Nadav: #1}}
\newcommand{\edo}[1]{\textcolor{orange}{Edo: #1}}
% If your paper is accepted, change the options for the package
% aistats2022 as follows:
%
\usepackage[accepted]{aistats2022}
%
% This option will print headings for the title of your paper and
% headings for the authors names, plus a copyright note at the end of
% the first column of the first page.

% If you set papersize explicitly, activate the following three lines:
%\special{papersize = 8.5in, 11in}
%\setlength{\pdfpageheight}{11in}
%\setlength{\pdfpagewidth}{8.5in}

% If you use natbib package, activate the following three lines:
%\usepackage[round]{natbib}
%\renewcommand{\bibname}{References}
%\renewcommand{\bibsection}{\subsubsection*{\bibname}}

% If you use BibTeX in apalike style, activate the following line:
%\bibliographystyle{apalike}
\bibliographystyle{apalike}

% a few useful commands
\newtheorem{theorem}{Theorem}[section]
\newtheorem{corollary}{Corollary}[theorem]
\newtheorem{lemma}[theorem]{Lemma}
\newtheorem{proposition}[theorem]{Proposition}
\newtheorem{definition}{Definition}[section]

\begin{document}

% If your paper is accepted and the title of your paper is very long,
% the style will print as headings an error message. Use the following
% command to supply a shorter title of your paper so that it can be
% used as headings.
%
%\runningtitle{I use this title instead because the last one was very long}

% If your paper is accepted and the number of authors is large, the
% style will print as headings an error message. Use the following
% command to supply a shorter version of the authors names so that
% they can be used as headings (for example, use only the surnames)
%
%\runningauthor{Surname 1, Surname 2, Surname 3, ...., Surname n}

% Supplementary material: To improve readability, you must use a single-column format for the supplementary material.
\onecolumn
% \aistatstitle{Instructions for Paper Submissions to AISTATS 2022: \\
% Supplementary Materials}

\aistatstitle{Supplementary Information for ``On the Implicit Bias of Gradient Descent for Temporal Extrapolation''}

\input{appendix/appendix_proofs}
\input{appendix/appendix_mimo} 
\input{appendix/appendix_experiments}
% \bibliography{refs}
% \section{FORMATTING INSTRUCTIONS}

% To prepare a supplementary pdf file, we ask the authors to use \texttt{aistats2022.sty} as a style file and to follow the same formatting instructions as in the main paper.
% The only difference is that the supplementary material must be in a \emph{single-column} format.
% You can use \texttt{supplement.tex} in our starter pack as a starting point, or append the supplementary content to the main paper and split the final PDF into two separate files.

% Note that reviewers are under no obligation to examine your supplementary material.

% \section{MISSING PROOFS}

% The supplementary materials may contain detailed proofs of the results that are missing in the main paper.

% \subsection{Proof of Lemma 3}

% \textit{In this section, we present the detailed proof of Lemma 3 and then [ ... ]}

% \section{ADDITIONAL EXPERIMENTS}

% If you have additional experimental results, you may include them in the supplementary materials.

% \subsection{The Effect of Regularization Parameter}

% \textit{Our algorithm depends on the regularization parameter $\lambda$. Figure 1 below illustrates the effect of this parameter on the performance of our algorithm. As we can see, [ ... ]}

% \vfill

\end{document}
